# Supplementary material for: Concentration of multi-overlaps for random ferromagnetic spin models
Source: arXiv:1901.06521 source file (2019-01-19)
Supplement: Supplementary file 1 [file appendix-proof-of-coupled-equiv.tex]

\section{Properties of the replica symmetric functionals}\label{proof:h_RS_coupled:equivalence}

In this appendix we collect a few useful structural properties of the replica symmetric functional. We start with the functional
\eqref{eq:RSFreeEntropy1} and then turn our attention to the interpolating one \eqref{eq:RSFreeEntropy_coupled1}.

We introduce a very convenient formalism which expresses these functionals in terms of a 
 a primary "entropy functional" and two types of convolution operations. This formalism first originated in the theory of error correcting codes \ref{ModernCodingBook} and turns out to be natural in the present context also. In fact we could have defined the RS functionals at the outset in this formalism.
Let $m(da)$ be a generic probability measure over $\overline{\mathbb{R}}_{+}$. We define an {\it entropy functional} $H: m \to \mathbb{R}$ as 
\begin{align}
H(m) = \int_{\overline{\mathbb{R}}} \ln (1+e^{-2 a}) m(a) da
\end{align}
There are two natural {\it convolution} operations $\circledast, \boxast$ defined as follows. For $a_1 \sim m_1, a_2 \sim m_2$, 
the usual convolution $m_1 \circledast m_2$ is the distribution of $a_1+a_2$; and $m_1 \boxast m_2$ is the distribution of $\tanh^{-1} (\tanh a_1 \tanh a_2)$. These convolution operations are commutative and associative. The mass $\delta_0$ at $a=0$ is the identity for $\circledast$ and is absorbing for $\boxast$. The mass at $\delta_{\infty}$ at $+\infty$ is the identity for $\boxast$ and is absorbing for $\circledast$. It is not difficult to see that
\begin{align}
H(\circledast_{i=1}^k m_i ) &  = \int \ln \big(1+e^{-2 \sum_{i=1}^k a_i}\big) \prod_{i=1}^k m_i (da_i) 
 \\
H(\boxast_{i=1}^k m_i ) & = - \int \ln \Big [ \frac{1}{2} \Big( 1 + \prod_{i=1}^k \tanh a_i \Big ) \Big ] \prod_{i=1}^k m_i (da_i).
\end{align}
Note that $H$ is commutative and associative under $\circledast$ and $\boxast$.
We define $\sfx_1^{\circledast 0} \equiv \Delta_0$, where $\Delta_0$ is the identity of $\circledast$. 

In the present problem 
all the measures involved are  $\sfx$, $\tilde{\sfx}$, or their "convolutions" and 
two point masses $\delta_J$, $\delta_H$ at $J$ and $H$. We introduce the notations $\tilde\sfx^{\boxast K} = \tilde\sfx \boxast \cdots \boxast \tilde\sfx$ ($K$ times), 
$\sfx^{\circledast l} = \sfx \circledast \cdots \circledast \sfx$ ($l$ times) 
and $\Lambda^\circledast(\sfx) = \sum_{l=0}^{+\infty} \frac{(\gamma p)l}{l!} e^{-\gamma p} \sfx^{\circledast l}$.
Recall that $U\sim \sfx$ and $V\sim \tilde\sfx$. 
It is not difficult to check that
\begin{align}
\mathbb{E} \ln \Big[ \frac{1}{2}( 1 + \tanh U \tanh V \Big ] = - H(\tilde\sfx\boxast\sfx)
\end{align}
\begin{align}
\mathbb{E} \ln \Big [\frac{1}{2}( 1 + \tanh \tJ \prod_{i=1}^{p}\tanh V_i )\Big] = - H(\delta_J\boxast \sfx^{\boxast p})
\end{align}
\begin{align}
\mathbb{E} \ln \Big [ e^{H} \prod_{b=1}^{l} (1 + \tanh U_b ) + e^{-H} \prod_{b=1}^{l} (1 - \tanh U_b ) \Big]
=
H(\delta_H \circledast \Lambda^{\circledast}(\tilde{\sfx})) - \gamma p H(\tilde{\sfx})
\end{align}
thus the  replica symmetric functional \eqref{eq:RSFreeEntropy1} becomes (up to a constant term)
\begin{align}
p_{\mathrm{RS}} ( \sfx, \tilde{\sfx} ) = H(\delta_H \circledast \Lambda^{\circledast}(\tilde{\sfx})) - \gamma p H(\tilde{\sfx})
-\gamma H(\delta_J\boxast \sfx^{\boxast p}) + \gamma p H(\tilde\sfx\boxast\sfx)  + {\rm constant}
\end{align}
This formalism makes it clear that: (i) the functional $\sfx\mapsto p_{\mathrm{RS}} ( \sfx, \tilde{\sfx} )$ (for fixed $\tilde\sfx$) is convex;
and similarly the functional $\tilde\sfx\mapsto p_{\mathrm{RS}} ( \sfx, \tilde{\sfx} )$ (for fixed $\sfx$) is convex. To see this one first notes that by linearity of $H$ both statements are true for the part $\gamma p H(\tilde\sfx\boxast\sfx)$. Let us prove that the term
$-\gamma H(\delta_J\boxast \sfx^{\boxast p})$ is convex.

% \begin{align}\label{eq:RSFreeEntropy1}
% p_{\mathrm{RS}} ( \sfx, \tilde{\sfx} ) 
% 	& = \mathbb{E} \ln \Big ( e^{H} \prod_{b=1}^{l} (1 + \tanh U_b ) + e^{-H} \prod_{b=1}^{l} (1 - \tanh U_b ) \Big) \-
% 	+ \gamma \mathbb{E} \ln \Big ( 1 + \tanh \tJ \prod_{i=1}^{p}\tanh V_i \Big)  \nonumber \\
% 	& \hspace{2cm} - p\gamma \mathbb{E} \ln \Big ( 1 + \tanh U \tanh V \Big )\-
% 	+ \gamma \ln \cosh \tJ\,.
% \end{align}
% 
% 
% 
% \begin{align}
% &{p}_{T}( \underline{\sfx}, \underline{\tilde{\sfx}}; h_0, \alpha  ) 
% 	=\E\ln \Big( e^{H + h_0 + h_1 \tau } \prod_{t=1}^{T} \prod_{b=1}^{l^{(t)}} (1 + \tanh U_b^{(t)} ) + e^{-H -h_0 - h_1\tau} \prod_{t=1}^{T} \prod_{b=1}^{l^{(t)}} (1 - \tanh U_b^{(t)} ) \Big) \nonumber \\
% 	& \quad + \frac{\gamma}{T} \sum_{t=1}^{T} \E\ln \Big( 1 + \tanh \tJ \prod_{i=1}^{p} \tanh V_i^{(t)} \Big) \-
% 	 - \frac{\gamma p}{T} \sum_{t=1}^{T}\E \ln \Big( 1 + \tanh U^{(t)} \tanh V^{(t)} \Big)  + \gamma \ln \cosh \tJ\,.
% \label{eq:RSFreeEntropy_coupled1}
% \end{align}

We also define $\Lambda^{\circledast}(\sfx_1) \equiv \sum_{l=0}^{\infty} \Lambda_l \sfx_1^{\circledast l}$, where $\Lambda_l = \frac{K^l e^{-K/R}}{R^l l!}$ denotes the probability that a variable node has degree $l$, and $\lambda^{\circledast}(\sfx_1) \equiv  \sum_{l=1} \lambda_l \sfx_1^{\circledast (l-1)}$, where $\lambda_l = \frac{i \Lambda_l}{\Lambda'(1)} = \frac{K^l e^{-K/R}}{R^l l!}$ denotes the probability that an edge is connected to a variable node of degree $l$. Let $\sfc$ be a distribution with only a point mass at $\tJ$ and $\sfh$ be a distribution with only a point mass at $h$.
One can check that
\begin{align}
\tilde{f} \big ( \underline{\sfx}, \underline{\tilde{\sfx}} \big ) 
	& = - \frac{K}{R} H \Big ( \frac{1}{T} \sum_{t=1}^{T} \tilde{\sfx}^{(t)} \Big  ) + H \Big  ( \sfh \circledast \Lambda^{\circledast} \Big ( \frac{1}{T} \sum_{t=1}^{T} \tilde{\sfx}^{(t)} \Big  ) \Big  ) \nonumber \\
	& \hspace{1cm} - \frac{1}{RT} \sum_{t=1}^{T} H \big (\sfc \boxast (\sfx^{(t)})^{\boxast K} \big ) + \frac{K}{RT} \sum_{t=1}^{T} H \big ( \tilde{\sfx}^{(t)} \boxast \sfx^{(t)} \big ) + \frac{1}{R} \ln \cosh \tJ + \frac{\ln 2}{R} + h.
\label{eq:RSFreeEntropy_coupled2}
\end{align}
The directional derivative of a function $F: \mathcal{P} \rightarrow \mathbb{R}$ at $\sfx_1$ in the direction $\Delta\sfx_1$ is
\begin{align*}
d_{\sfx_1} F(\sfx_1) [\Delta \sfx_1] \equiv \lim_{\delta \rightarrow 0} \frac{F(\sfx_1 + \Delta \sfx_1) - F(\sfx_1)}{\delta}.
\end{align*}
The stationary condition is then given by $d_{\tilde{\sfx}^{(t)}} \tilde{f}(\underline{\sfx}, \underline{\tilde{\sfx}})[\Delta \sfx^{(t)}] = 0$ and $d_{\sfx^{(t)}} \tilde{f}(\underline{\sfx}, \underline{\tilde{\sfx}})[\Delta \sfx^{(t)}] = 0$. 
To compute them we employ the following computational rules known in literature.

\begin{lemma}%[{\cite[Propositions 14 and 15]{KumYMP:2014}}]
Let $F: \mathcal{P} \rightarrow \mathbb{R}$ be a linear functional, and $*$ be either $\circledast$ or $\boxast$. Then for $k \in \mathbb{Z}^{+}$, $\sfx_1, \sfx_2, \sfx'_2 \in \mathcal{P}$ and letting $\sfy = \sfx_2 - \sfx'_2$, we have
\begin{align*}
d_{\sfx_1} F(\sfx_1^{* k})[\sfy] = k F(\sfx_1^{* (k-1)} * \sfy).
\end{align*}
For any polynomials $p,q$, we have
\begin{align*}
d_{\sfx_1} F \big (p^{\circledast}(q^{\boxast}(\sfx)) \big )[\sfy] = F \big ( p'^{\circledast}(q^{\boxast}(\sfx_1) \circledast (q'^{\boxast}(\sfx_1) \boxast \sfy )\big ).
\end{align*}
\label{thm:entropyFunctional:derivative}
\end{lemma}

\begin{lemma}%[{\cite[Theorem 4.41]{MCT:2008}}]
For any $\sfx_1, \sfx'_1, \sfx_2 \in \mathcal{P}$, we have
\begin{align*}
H((\sfx_1 - \sfx'_1)\circledast \sfx_2) + H((\sfx_1 - \sfx'_1) \boxast \sfx_2) = H(\sfx_1 - \sfx'_1).
\end{align*}
\label{thm:entropyFunctional:duality}
\end{lemma}

Let $\sfT(\underline{\tilde{\sfx}}) \equiv \sfh \circledast \lambda^{\circledast} \left ( \frac{1}{T} \sum_{t=1}^{T} \tilde{\sfx}^{(t)} \right )$. Using Lemma~\ref{thm:entropyFunctional:derivative}, $d_{\tilde{\sfx}^{(t)}} \tilde{f}(\underline{\sfx}, \underline{\tilde{\sfx}})[\Delta \tilde{\sfx}^{(t)}]$ is the sum of the following terms:
\begin{align}
- d_{\tilde{\sfx}^{(t)}} \frac{K}{R} H \Big ( \frac{1}{T} \sum_{t=1}^{T} \tilde{\sfx}^{(t)} \Big  ) [\Delta \tilde{\sfx}^{(t)}]
	& = - \frac{K}{RT}
			H  ( \Delta \tilde{\sfx}^{(t)} )\,,\label{eq:dir_derivative:term1}\\
d_{\tilde{\sfx}^{(t)}} H \Big ( \sfh \circledast \Lambda^{\circledast}\Big ( \frac{1}{T} \sum_{t=1}^{T} \tilde{\sfx}^{(t)} \Big) \Big) [\Delta \tilde{\sfx}^{(t)}]
	& = \frac{K}{RT} H ( \sfT(\underline{\tilde{\sfx}}) \circledast \Delta \tilde{\sfx}^{(t)}), \label{eq:dir_derivative:term2}\\
- d_{\tilde{\sfx}^{(t)}} \frac{K}{RT} \sum_{t=1}^{T} H \big (\sfx^{(t)} \boxast \sfx^{(t)} \big ) [\Delta \tilde{\sfx}^{(t)}]
	& = - \frac{K}{RT} H  ( \Delta \tilde{\sfx}^{(t)} \boxast \sfx^{(t)}  ), \label{eq:dir_derivative:term3}
\end{align}
In addition, we use Lemma~\ref{thm:entropyFunctional:duality} to rewrite \eqref{eq:dir_derivative:term2} as
\begin{align}
\frac{K}{RT} \big \{ H ( \Delta \tilde{\sfx}^{(t)} ) - H ( \sfT(\underline{\tilde{\sfx}}) \boxast \Delta \tilde{\sfx}^{(t)}  )   \big \}. \label{eq:dir_derivative:term2a}
\end{align}
Putting \eqref{eq:dir_derivative:term1}, \eqref{eq:dir_derivative:term3} and \eqref{eq:dir_derivative:term2a} together, we have
\begin{align*}
d_{\tilde{\sfx}^{(t)}} \tilde{f}(\underline{\sfx}, \underline{\tilde{\sfx}})[\Delta \tilde{\sfx}^{(t)}]
	& = \frac{K}{RT} H  ( \Delta \tilde{\sfx}^{(t)} \boxast (\sfx^{(t)} - \sfT(\underline{\tilde{\sfx}}) )  ),
	%\label{eq:dhcoupled_dxt}
\end{align*}
which implies that the stationary point of $\tilde{f}(\underline{\sfx}, \underline{\tilde{\sfx}})$ is attained at $\sfx^{(t)} = \sfT(\underline{\tilde{\sfx}})$ for all $t$.

Let $\tilde{\sfT}(\sfx^{(t)}) = \sfc \boxast (\sfx^{(t)})^{\boxast (K-1)}$. The same kind of calculation with the use of Lemma~\ref{thm:entropyFunctional:derivative} gives
\begin{align*}
d_{\sfx^{(t)}} \tilde{f} ( \underline{\sfx}, \underline{\tilde{\sfx}}) [\Delta \sfx^{(t)}]
	& = \frac{K}{RT} H ( \Delta \sfx^{(t)} \boxast ( \tilde{\sfT}(\sfx^{(t)}) - \tilde{\sfx}^{(t)} ) ).
\end{align*}
The stationary point of $\tilde{f}(\underline{\sfx}, \underline{\tilde{\sfx}})$ is attained at $\tilde{\sfx}^{(t)} = \tilde{\sfT}(\sfx^{(t)}) = \tilde{\sfT}(\sfT(\underline{\tilde{\sfx}}))$ for all $t$.
