# Supplementary material for: Concentration of multi-overlaps for random ferromagnetic spin models
Source: arXiv:1901.06521 source file (2019-01-19)
Supplement: Supplementary file 2 [file appendix-removeperturbation.tex]

\section{Removing the perturbations}\label{elementaryapp}
\begin{lemma}
 Let $F_n: [0,1] \to \mathbb{R}_{+}$ be a sequence of non-negative continuous functions. Suppose that 
 $$
 \lim_{n\to \infty} \int_0^1 d\epsilon F_n(\epsilon) = 0\,.
 $$
 Given any $\bar \epsilon \in [0,1]$ we can find a sequence $\epsilon_n \to \bar \epsilon$, $n\to \infty$ such that $\lim_{n\to \infty} F_n(\epsilon_n) =0$. 
\end{lemma}
\begin{proof}
Set $a_n = \sqrt{\int_0^1 d\epsilon F_n(\epsilon)}$. First we consider the case $\bar \epsilon \in ]0,1[$. Note that $\lim_{n\to \infty} a_n =0$ so for $n$ large enough
$[\bar \epsilon - a_n , \bar \epsilon +a_n] \subset [0,1]$ and thus
\begin{align*}
 \int_0^1 d\epsilon F_n(\epsilon) \geq \int_{\bar \epsilon - a_n}^{\bar \epsilon +a_n} d\epsilon F_n(\epsilon)\,. 
\end{align*}
The mean value theorem tells us that there exists $\epsilon_n \in [\bar \epsilon - a_n, \bar \epsilon +a_n]$ such that the right hand side equals 
$2a_n F_n(\epsilon_n)$. Therefore dividing both sides of the previsou inequality by $2a_n$ we obtain
\begin{align*}
 0\leq F_n(\epsilon_n) \leq \frac{1}{2} \sqrt{\int_0^1 d\epsilon F_n(\epsilon)}
\end{align*}
which implies the claim for $\bar \epsilon \in ]0,1[$. Now we consider $\bar\epsilon =0$. Similarly as before we have for $n$ large enough
\begin{align*}
 \int_0^1 d\epsilon F_n(\epsilon) \geq \int_{0}^{a_n} d\epsilon F_n(\epsilon) = a_n F_n(\epsilon_n)\,. 
\end{align*}
for some $\epsilon_n$ by the mean value theorem. This implies $0\leq F_n(\epsilon_n) \leq \sqrt{\int_0^1 d\epsilon F_n(\epsilon)}$ and the claim follows. The case $\bar\epsilon=1$ is treated in the same way.
\end{proof}
The whole point of this lemma is that although the functions $F_n$ are uniformly bounded we might not a priori know if their pointwise limit exists almost everywhere and thus, in this case, we cannot use Lebesgue's dominated convergence theorem while this lemma can be used.
