# Supplementary material for: Concentration of multi-overlaps for random ferromagnetic spin models
Source: arXiv:1901.06521 source file (2019-01-19)
Supplement: Supplementary file 3 [file appendix-equivalence.tex]

\section{appendix-equivalence}\label{appendix-equivalence}
